# Supplementary material for: Machine Learned Learning Machines
Source: arXiv:1705.10201 ancillary file (2017-08-31)
Supplement: Supplementary file 1 [file Supplementary.pdf]

# Supplementary Material

Leigh Sheneman

Department of Computer Science and Engineering,  
Michigan State University  
BEACON-Center for the Study of Evolution in Action,  
Michigan State University

Arend Hintze

Department of Integrative Biology Michigan State University  
Department of Computer Science and Engineering,  
Michigan State University  
BEACON-Center for the Study of Evolution in Action,  
Michigan State University

August 31, 2017

## 1 Minimum Performance Distribution

For each evolutionary experimental condition, we recorded the minimum number of times each of the 300 agents reached the goal across all 24 maps. We see that minimum number of times an agent reaches the goal has a left-skewed distribution in all three treatments, indicating that learning the task is non-trivial.

## 2 Feedback Integration

Agents that were evolved using feedback gates have the potential to change their probability table within their lifetime. By computing the difference between the ables from each feedback gate at birth and after 512 updates,

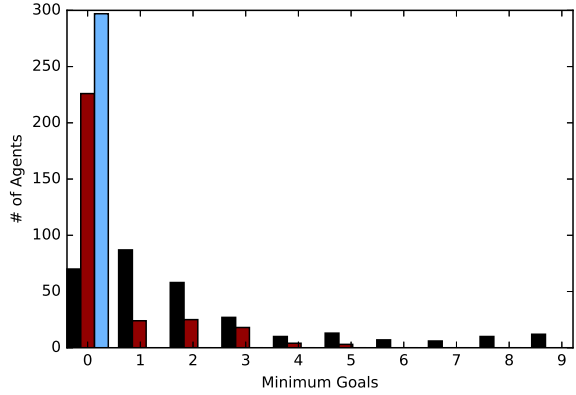

Figure 1: Minimum Performance Distribution for three experimental conditions. Black all gates allowed, blue deterministic and probabilistic gates allowed, red only deterministic gates.

we find that indeed these tables change over their lifetime, but this difference neither increases or decreases over evolutionary time (see Figure 2). The difference was computed using the root mean square method. In addition, we find only a very weak correlation between the amount of change and performance (see Figure 3).

### 3 Computational Networks

When we compare the behavior of the best performing agent using feedback gates, with that of the best performing agent that does not use feedback gates, we find one very striking difference. To exemplify this we show the best performing agent without feedback gates (see Figure 5) to developed a complex network of deterministic gates (shown with square boxes) and seem to make use of the hidden nodes of the Markov Brain. While the best performing agent that has feedback gates (see Figure 4), seems to write to the hidden states less and both output nodes receive a signal from the feedback gate (seen in the octagon).

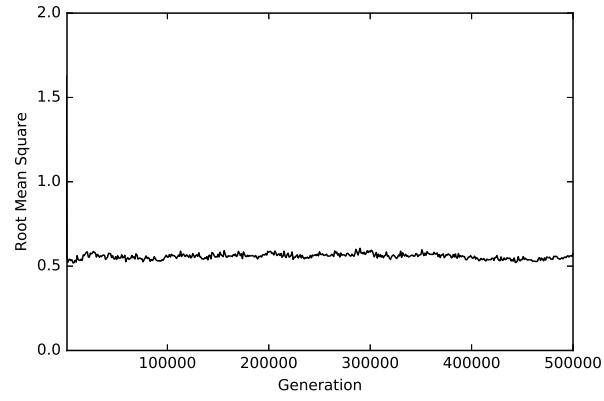

Figure 2: Root mean square difference between probability tables at birth and after learning is over for each generation on the LOD.

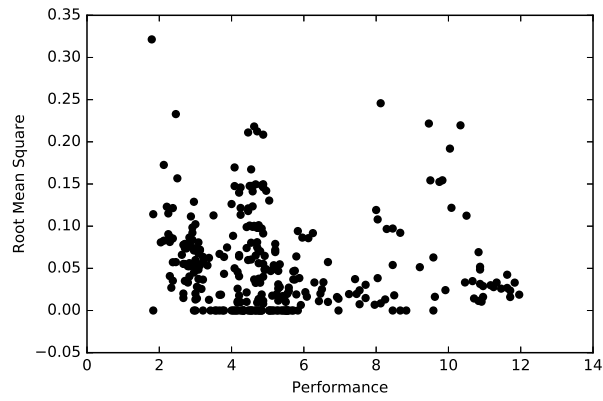

Figure 3: Correlation of change in root mean square to performance at the end of evolution.

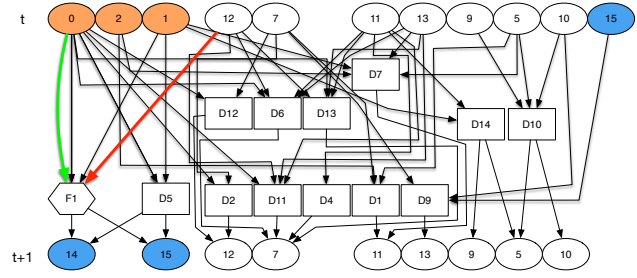

Figure 4: Computational network of best performing agent using feedback. Input nodes are orange, output nodes are blue, hidden nodes are white. Positive feedback connections are green arrows, and negative feedback are red arrows. Logic gates are rectangular boxes, while the feedback gate is an octagon. The top row of nodes represents the states at time point  $t$ , while the bottom row of nodes represents the internal states of the Markov Brain at time point  $t + 1$ .

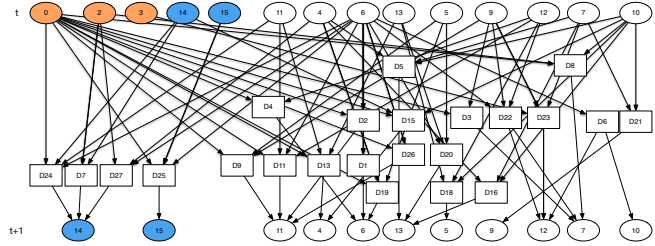

Figure 5: Computational network of best performing agent not using feedback. Input nodes are orange, output nodes are blue, hidden nodes are white, logic gates are rectangular boxes. The top row of nodes represents the states at time point  $t$  while the bottom row of nodes represents the internal states of the Markov Brain at time point  $t + 1$ .

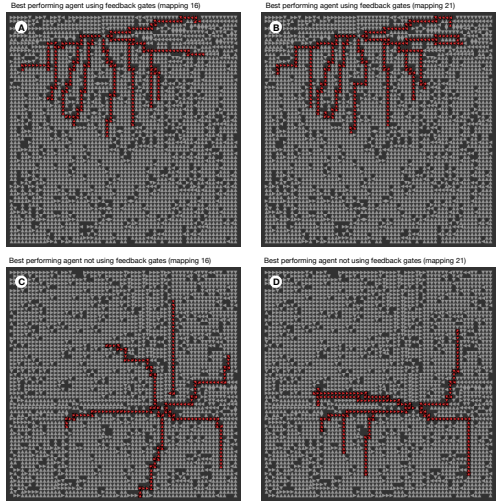

Figure 6: Path comparison of the best performing feedback agent versus best performer without feedback.

## 4 Performance Plots

Each image depicts an environment where the cells are labeled using a gray arrow, pointing towards the optimal path. Dark gray boxes are walls or obstacles in the environment. The red arrows indicate the orientation and location an agent had during its life. Once agents reached the goal, they were put back to a random location 23 steps away from the goal. The left two images, labeled A and C, depict the path in environment 16, and the right two images, labeled B and D, show environment 21. We see that either evolved agent moves on a straight line without attempting to take turns when they move on a straight line of forward facing arrows. However, the agent using feedback gates makes less mistakes when it comes to turns, whereas the agent not using feedback gates struggles to find the correct direction at every turn, and also reaches the goal less often.

## 5 Average Updates to Goals

For the top 50 performing agents using all three types of gates—deterministic, probabilistic, and feedback gates—we recorded the number of updates it takes

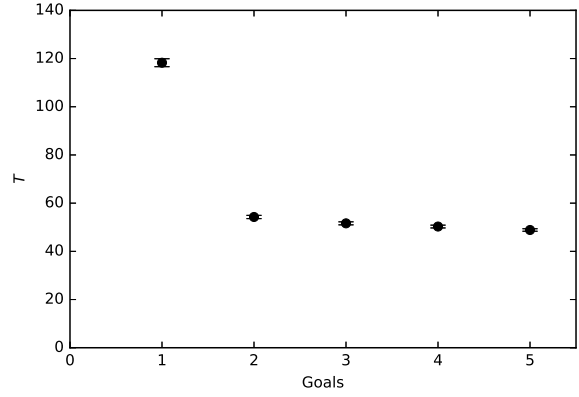

Figure 7: Average updates required to reach first five goals.

to get to the first five goals. This allows us to estimate the progression of learning. We find that the time to reach the first goal takes about 118 steps, to the next one only 54, and finally this trend stabilizes at about 50 steps to the goal.

## 6 Learning a Single Map

To create a fair comparison between  $Q$ -learning and MBs we evolved 300 replicates of MBs to solve one map for 5,000 generations. Here we plot the mean performance over evolutionary time for agents on the LOD. Agents where able to match the performance of the  $Q$ -learners less than 400 generations.

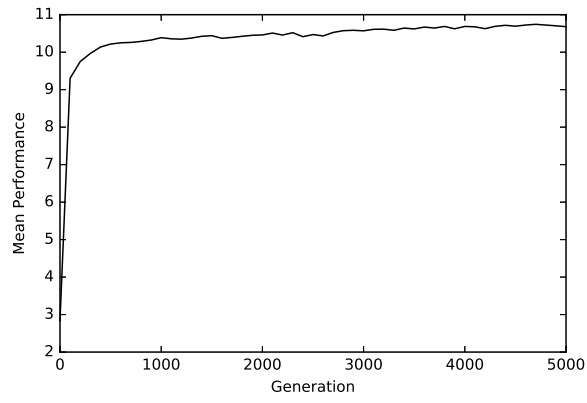

Figure 8: Performance over evolutionary time when evolved on a single map.
